# Supplementary material for: SemRob: Towards Semantic Stream Reasoning for Robotic Operating Systems
Source: arXiv:2201.11625 source file (2022-01-27)
Supplement: Supplementary file 1 [file appendix.tex]

\section*{Appendix}
\addcontentsline{toc}{section}{Appendix}
When placed at the end of a chapter or contribution (as opposed to at the end of the book), the numbering of tables, figures, and equations in the appendix section continues on from that in the main text. Hence please \textit{do not} use the \verb|appendix| command when writing an appendix at the end of your chapter or contribution. If there is only one the appendix is designated ``Appendix'', or ``Appendix 1'', or ``Appendix 2'', etc. if there is more than one.

\begin{equation}
a \times b = c
\end{equation}
